# Supplementary material for: PANORAMIA: Privacy Auditing of Machine Learning Models without Retraining
Source: arXiv:2402.09477 source file (2024-10-26)
Supplement: Supplementary file 1 [file extra_results.tex]

\section{Additional Results}

\begin{figure*}
  \centering
  \subfigure[Privacy Audit of the ResNet101 at varying degrees of training on the CIFAR10  image dataset.]{\includegraphics[width=0.31\textwidth]{images/Res101_NEW_Mean_ROC_Curves-Dataset_Size_2820.pdf}}
  \hfill
  \subfigure[Privacy Audit of the Wide ResNet-28-2 at varying degrees of training on the CIFAR10 image dataset.]{\includegraphics[width=0.31\textwidth]{images/Wide-28-2Mean_ROC_Curves-Dataset_Size_2220.pdf}}
  \hfill
  \subfigure[Privacy Audit of a Multi-Label CNN at varying degrees of training on the CelebA image dataset.]{\includegraphics[width=0.34\linewidth]{images/CelebA_wide_Mean_ROC_Curves-Dataset_Size2220.pdf}}
  \caption{Comparison of our privacy auditing mechanism with target models (\model) as ResNet101 and WideResNet-28-2 models, on CIFAR10 dataset and Multi-Label CNN model on the CelebA dataset at varying degrees of training and overfitting.}\label{fig:overfitting_comparison}
 
\end{figure*}
\begin{figure}[h]
    \centering
     \subfigure[Privacy audit of a three hidden-layers neural network on the Adult dataset.]
      {\includegraphics[width=0.21\textwidth]{images/Tab_Results_Overfit.pdf}}  
    \hfill
     \subfigure[Privacy audit of GPT-2 on the wiki-text dataset, trained on a varying number of epochs.]
        {\includegraphics[width=0.21\textwidth]{images/Tab_Results_Overfit.pdf}}
    \caption{Comparison of our privacy auditing mechanism with target models (\model) as ResNet101 and WideResNet-28-2 models, on CIFAR10 dataset and Multi-Label CNN model on the CelebA dataset at varying degrees of training and overfitting.}\label{fig:overfitting_tab_nlp}    
\end{figure}

\begin{figure}[tbp]
  \centering  
\includegraphics[width=0.4\textwidth]{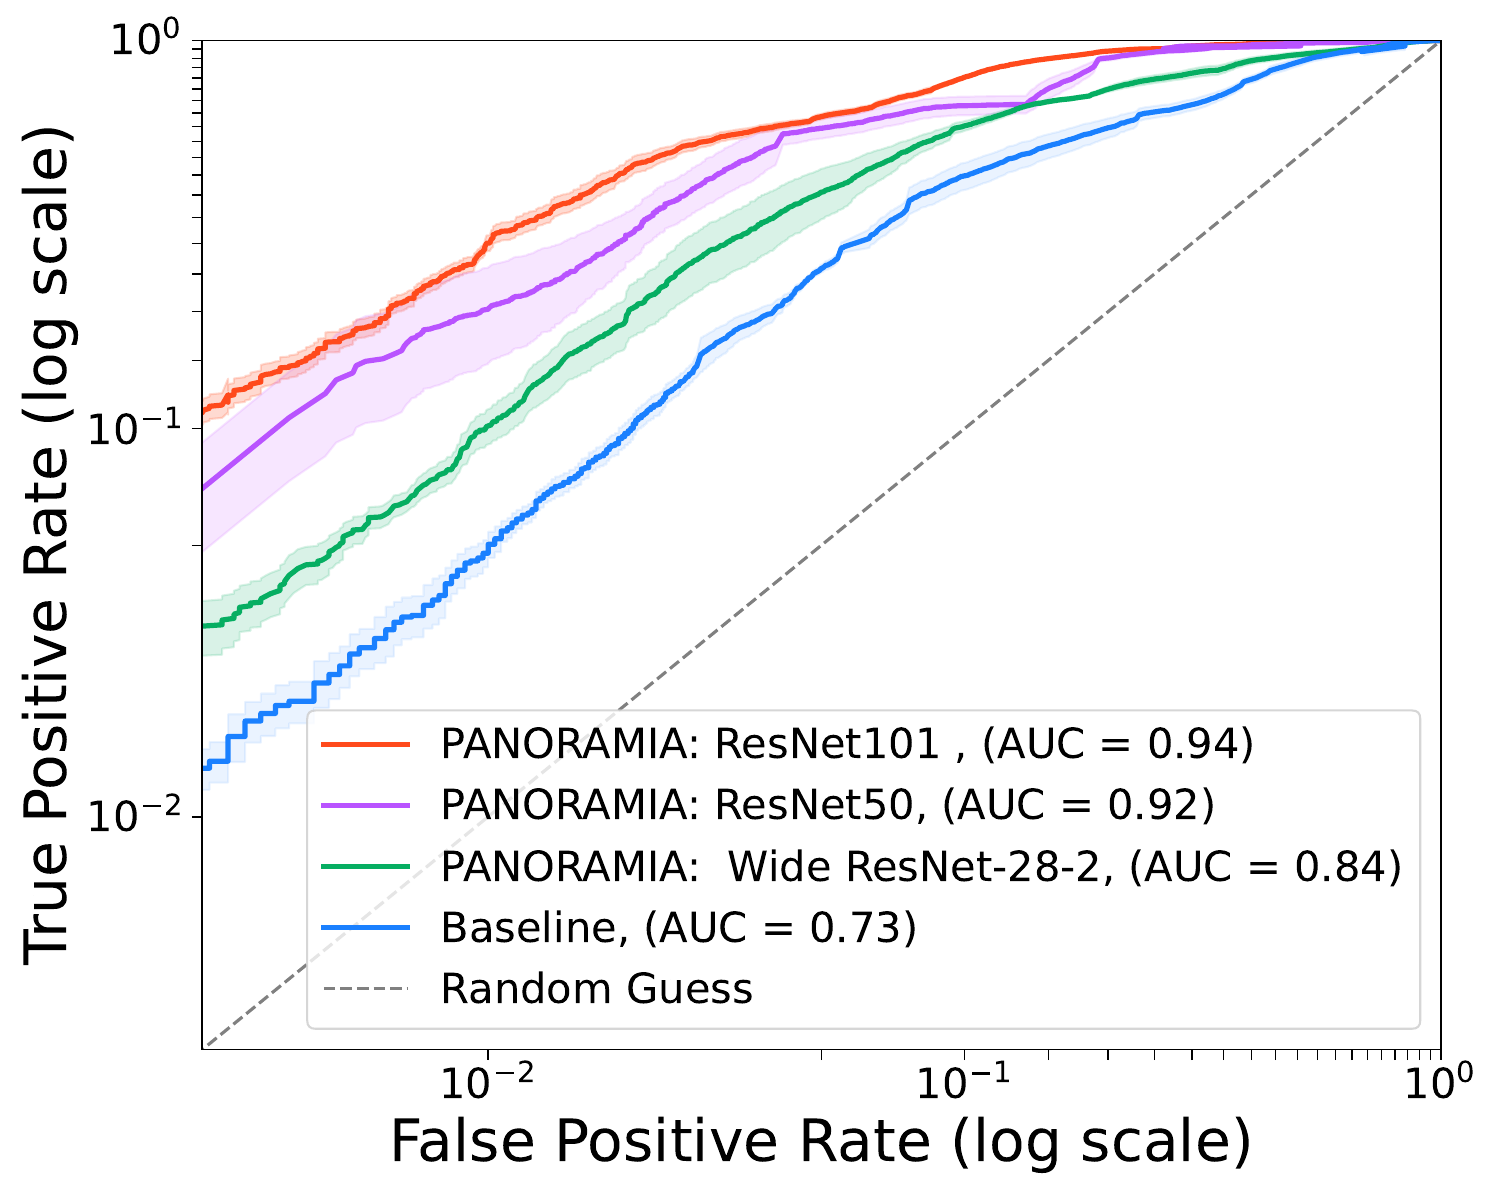}
  \caption{A comparison of three different image classification target models trained on the CIFAR10 dataset. We show the privacy audit of these models in varying degrees of complexity, with Wide ResNet-28-2 being the least complex, followed by ResNet 50, and finally ResNet101. All models are generalized models (no overfitting).}
  \label{fig:complex_model}
\end{figure}
